# Supplementary material for: SHAPO: Sharpness-Aware Policy Optimization for Safe Exploration
Source: arXiv:2606.10228 source file (2026-06-08)
Supplement: Supplementary file 2 [file appendix_old.tex]

\appendix
\section{Technical Appendix: Detailed Proofs and Derivations}
\label{app:proofs}

\subsection{Assumptions and Notation}
\label{app:assumptions}
We assume throughout:
\begin{enumerate}
\item (Regularity) $\mathcal{L}_\lambda$ is $C^2$ in a neighborhood of the iterates, with locally Lipschitz Hessian, i.e., there exists $L_3(\theta)>0$ s.t.\ $\| \nabla^2 \mathcal{L}_\lambda(\theta+\Delta)-\nabla^2 \mathcal{L}_\lambda(\theta)\| \le L_3(\theta)\|\Delta\|$.
\item (Fisher PD) The (empirical) Fisher $F(\theta)$ in \eqref{eq:fisher} is positive definite (or damped $F_\varepsilon:=F+\varepsilon I\succ 0$ with small $\varepsilon>0$), and the local KL expansion \eqref{eq:kl-local} holds.
\item (On-policy surrogates) Expectations defining $g(\theta)$ and $F(\theta)$ are taken under the current on-policy distribution, computed from finite trajectories with standard variance-reduction baselines.
\end{enumerate}
For a symmetric PD matrix $A$, define the (semi)norms $\|x\|_{A}:=\sqrt{x^\top A x}$ and $\|x\|_{A^{-1}}:=\sqrt{x^\top A^{-1} x}$. We denote $g:=\nabla_\theta \mathcal{L}_\lambda(\theta)$ and $H:=\nabla_\theta^2 \mathcal{L}_\lambda(\theta)$ for brevity, and drop the explicit $(\theta)$ when clear.

\subsection{Preliminaries: KL Geometry and Dual Norm}
\label{app:prelim}
The average KL ball around $\pi_\theta$ is locally the Fisher ellipsoid
\[
\mathcal{E}_\rho \;:=\; \Big\{ \Delta \in \mathbb{R}^p \;:\; \tfrac{1}{2}\Delta^\top F \Delta \le \rho \Big\}.
\]
The support function of $\mathcal{E}_\rho$ in direction $g$ equals $\sqrt{2\rho}\,\|g\|_{F^{-1}}$. This is a standard dual-norm identity:
\[
\sup_{\Delta \in \mathcal{E}_\rho} g^\top \Delta
= \sup_{\|\Delta\|_F \le \sqrt{2\rho}} \langle g, \Delta \rangle
= \sqrt{2\rho}\, \|g\|_{F^{-1}} \quad\text{(Cauchy--Schwarz in the $F$-inner product)}.
\]
We give a full KKT derivation in Lemma~\ref{lem:app-inner}.

\subsection{Proof of Lemma~\ref{lem:inner-max-linear} (Inner maximization over Fisher ellipsoid)}
\label{app:proof-lem1}

Under the first-order model $\mathcal{L}_\lambda(\theta+\Delta)\approx \mathcal{L}_\lambda(\theta)+g^\top \Delta$
and constraint $\frac{1}{2}\Delta^\top F \Delta \le \rho$ with $F\succ 0$, the inner maximization has the unique optimizer
\[
\Delta^\star = \sqrt{2\rho}\,\frac{F^{-1}g}{\|g\|_{F^{-1}}}, \qquad
\max_{\Delta} g^\top \Delta = \sqrt{2\rho}\,\|g\|_{F^{-1}}.
\]


\begin{proof}
Consider the convex program
\[
\max_{\Delta} \;\; g^\top \Delta \quad \text{s.t.}\quad \tfrac{1}{2}\Delta^\top F \Delta \le \rho.
\]
Slater holds (e.g., $\Delta=0$ is strictly feasible if $\rho>0$), so strong duality applies. The Lagrangian is
\[
\mathcal{J}(\Delta,\eta) = g^\top \Delta - \eta\left(\tfrac{1}{2}\Delta^\top F \Delta - \rho\right),
\quad \eta\ge 0.
\]
KKT conditions: (i) stationarity: $\nabla_\Delta \mathcal{J} = g - \eta F \Delta = 0$,
so $\Delta = \eta^{-1}F^{-1} g$; (ii) complementary slackness: $\eta\left(\tfrac{1}{2}\Delta^\top F \Delta - \rho\right)=0$; (iii) primal feasibility: $\tfrac{1}{2}\Delta^\top F \Delta \le \rho$; (iv) dual feasibility $\eta\ge 0$.
For $g\neq 0$, at optimum we must have $\eta>0$ (otherwise the linear objective is unbounded), thus the constraint is tight:
\[
\tfrac{1}{2}\Delta^\top F \Delta = \tfrac{1}{2}\eta^{-2} g^\top F^{-1} g = \rho
\;\Rightarrow\;
\eta = \sqrt{\frac{g^\top F^{-1} g}{2\rho}}.
\]
Substitute into $\Delta$ to obtain $\Delta^\star = \sqrt{2\rho}\, F^{-1} g / \|g\|_{F^{-1}}$.
The optimal value is $g^\top \Delta^\star = \sqrt{2\rho}\, \|g\|_{F^{-1}}$.
Uniqueness follows from strict convexity of the constraint and linearity of the objective.
\end{proof}

\subsection{Proof of Theorem~\ref{thm:mean-std} (Mean--Std epistemic risk aversion)}
\label{app:proof-thm1}
With the second-order expansion
$\mathcal{L}_\lambda(\theta+\Delta)=\mathcal{L}_\lambda(\theta)+g^\top\Delta + \tfrac{1}{2}\Delta^\top H \Delta + R_3(\Delta)$,
the KL--SAM objective satisfies, locally,
\[
\max_{\frac{1}{2}\Delta^\top F \Delta \le \rho}\; \mathcal{L}_\lambda(\theta+\Delta)
= \mathcal{L}_\lambda(\theta) + \sqrt{2\rho}\,\|g\|_{F^{-1}} + \frac{1}{2}\Delta^{\star\top} H \Delta^\star + R_3(\Delta^\star),
\]
where $\Delta^\star$ is as in Lemma~\ref{lem:inner-max-linear}. Under a Laplace posterior
$\theta' \sim \mathcal{N}(\theta, F^{-1})$, the linearized loss variance is
$\mathrm{Var}[\mathcal{L}_\lambda(\theta')] = g^\top F^{-1} g$, so the first-order risk premium equals
$\sqrt{2\rho}\,\sqrt{\mathrm{Var}[\mathcal{L}_\lambda(\theta')]}$.

\begin{proof}
Taylor's theorem with integral remainder yields, for some $t\in(0,1)$,
\[
\mathcal{L}_\lambda(\theta+\Delta)
= \mathcal{L}_\lambda(\theta) + g^\top \Delta + \tfrac{1}{2}\Delta^\top H \Delta
+ \underbrace{\int_0^1 \tfrac{(1-t)^2}{2}\, \Delta^\top \nabla^3 \mathcal{L}_\lambda(\theta+t\Delta)[\Delta,\Delta] \, dt}_{=:R_3(\Delta)}.
\]
First, ignoring curvature and remainder, Lemma~\ref{lem:inner-max-linear} gives
$\max_{\mathcal{E}_\rho} \{\mathcal{L}_\lambda(\theta)+g^\top\Delta\} = \mathcal{L}_\lambda(\theta)+\sqrt{2\rho}\|g\|_{F^{-1}}$
attained at $\Delta^\star = \sqrt{2\rho}\,F^{-1}g/\|g\|_{F^{-1}}$.
Adding back the quadratic term at that $\Delta^\star$ produces
$\tfrac{1}{2}\Delta^{\star\top} H \Delta^\star$.
For the remainder, by the Lipschitz Hessian assumption there exists $L_3$ (local) such that
$\|R_3(\Delta)\| \le \tfrac{L_3}{6}\|\Delta\|^3$; since $\|\Delta^\star\| = \mathcal{O}(\sqrt{\rho})$
(precisely, $\|\Delta^\star\|\le \sqrt{2\rho}\,\|F^{-1}g\|/\|g\|_{F^{-1}}$), we get $R_3(\Delta^\star)=\mathcal{O}(\rho^{3/2})$.
Thus the first two correction terms in \eqref{eq:sam-mean-std} scale as $\mathcal{O}(\sqrt{\rho})$ and $\mathcal{O}(\rho)$, respectively, and the remainder is $o(\rho)$.

For the variance identity, linearize $\mathcal{L}_\lambda(\theta')\approx \mathcal{L}_\lambda(\theta)+g^\top(\theta'-\theta)$
with $\theta'-\theta\sim \mathcal{N}(0, F^{-1})$ under Laplace approximation; hence
$\mathrm{Var}[\mathcal{L}_\lambda(\theta')] \approx g^\top F^{-1} g$.
\end{proof}

\subsection{Curvature Correction as a Spectral Bound (Remark~\ref{rem:curvature})}
\label{app:curvature}
Let $M := F^{-1/2} H F^{-1/2}$ and write $\Delta^\star = \sqrt{2\rho}\,F^{-1/2} u$ with $u:=F^{-1/2}g/\|g\|_{F^{-1}}$ normalized so that $\|u\|_2=1$. Then
\[
\frac{1}{2}\Delta^{\star\top} H \Delta^\star
= \rho\, u^\top M u.
\]
By the Rayleigh quotient bounds,
$\lambda_{\min}(M) \le u^\top M u \le \lambda_{\max}(M)$, hence
\[
-\rho\,\|M\| \;\le\; \frac{1}{2}\Delta^{\star\top} H \Delta^\star \;\le\; \rho\,\|M\|,
\qquad \|M\|=\max\{|\lambda_{\min}(M)|,|\lambda_{\max}(M)|\}.
\]
Combining with the linear term yields \eqref{eq:upper-lower}.

\subsection{Second-Order Inner Maximization as a Trust-Region Subproblem}
\label{app:second-order-inner}
Consider the \emph{exact} inner problem with quadratic model:
\begin{equation}
\label{eq:quad-inner}
\max_{\frac{1}{2}\Delta^\top F \Delta \le \rho} \quad g^\top \Delta + \tfrac{1}{2}\Delta^\top H \Delta.
\end{equation}
This is a (concave) trust-region problem iff $H - \eta F \prec 0$ for the optimal dual variable $\eta$.
Form the Lagrangian $\mathcal{J}(\Delta,\eta)=g^\top \Delta + \tfrac{1}{2}\Delta^\top H \Delta - \tfrac{\eta}{2}(\Delta^\top F \Delta - 2\rho)$, with $\eta\ge 0$.
Stationarity gives $(H - \eta F)\Delta + g = 0 \Rightarrow \Delta(\eta) = - (H - \eta F)^{-1} g$ (well-defined for $\eta>\lambda_{\max}(F^{-1/2} H F^{-1/2})$).
Complementary slackness implies the constraint is tight for $g\neq 0$, so $\eta$ is the unique root of
\[
\phi(\eta) \;:=\; \tfrac{1}{2}\Delta(\eta)^\top F \Delta(\eta) - \rho \;=\; 0,
\qquad \eta>\lambda_{\max}(M),\; M=F^{-1/2} H F^{-1/2}.
\]
Thus the exact optimizer is
\[
\Delta^{\star}_{\text{quad}} \;=\; - (H - \eta^\star F)^{-1} g,
\quad \text{with }\eta^\star \text{ chosen so that } \tfrac{1}{2}\Delta^{\star\top}_{\text{quad}} F \Delta^{\star}_{\text{quad}} = \rho.
\]
The optimal value is
\[
g^\top \Delta^{\star}_{\text{quad}} + \tfrac{1}{2}\Delta^{\star\top}_{\text{quad}} H \Delta^{\star}_{\text{quad}}
= \rho\,\eta^\star \;-\; \tfrac{1}{2}\, g^\top (H - \eta^\star F)^{-1} g.
\]
As $\rho\downarrow 0$, one has $\eta^\star \to +\infty$ and
$\Delta^{\star}_{\text{quad}} \to \sqrt{2\rho}\,F^{-1}g/\|g\|_{F^{-1}}$, recovering Lemma~\ref{lem:inner-max-linear}.
This characterization justifies the curvature corrections reported in the main text and motivates practical damped Newton/natural-gradient solvers for the inner point.

\subsection{Calibration via Credible Sets: Proof of \eqref{eq:rho-alpha}}
\label{app:credible}
Under the Laplace approximation, the posterior over $\theta$ is $\mathcal{N}(\hat\theta, \Sigma)$ with $\Sigma=F(\hat\theta)^{-1}$.
The $(1-\alpha)$ credible ellipsoid centered at $\hat\theta$ is
\[
\mathcal{C}_\alpha \;=\; \Big\{ \theta: (\theta-\hat\theta)^\top \Sigma^{-1} (\theta-\hat\theta) \le \chi^2_{p}(1-\alpha) \Big\}.
\]
Parametrize $\Delta=\theta-\hat\theta$ and set $\tau:=\chi^2_{p}(1-\alpha)$.
Using the local KL identity \eqref{eq:kl-local}, the KL ball $\tfrac{1}{2}\Delta^\top F \Delta \le \rho$
corresponds to $\Delta^\top \Sigma^{-1}\Delta \le 2\rho$. Hence
\[
2\rho \;=\; \tau \;=\; \chi^2_{p}(1-\alpha)
\qquad\Longleftrightarrow\qquad
\rho \;=\; \tfrac{1}{2}\,\chi^2_{p}(1-\alpha).
\]
Writing the credible \emph{coverage} level as $\alpha_{\mathrm{cov}}:=1-\alpha$ recovers \eqref{eq:rho-alpha} (notation varies across texts). Consequently,
$\beta(\rho)=\sqrt{2\rho}=\sqrt{\chi^2_p(\alpha_{\mathrm{cov}})}$; in high dimensions one may substitute the Wilson--Hilferty approximation if desired.

\subsection{Epistemic vs.\ Aleatoric: Why the Penalty is Epistemic}
\label{app:epi-alea}
The Fisher $F(\theta)=\mathbb{E}_{s\sim d^\pi, a\sim \pi_\theta}[\nabla\log\pi_\theta \nabla\log\pi_\theta^\top]$ captures local sensitivity of the \emph{likelihood} to parameter changes, i.e., parameter uncertainty.
Under Laplace, $\Sigma \approx F^{-1}$ serves as a proxy posterior covariance: as data accumulates, $F$ grows and $\Sigma$ shrinks, so $\|g\|_{F^{-1}} \downarrow 0$.
By contrast, aleatoric noise (transition or reward stochasticity) affects gradient \emph{variance} but not the geometry $F^{-1}$ of the penalty; thus the $\sqrt{2\rho}\,\|g\|_{F^{-1}}$ term attenuates with epistemic uncertainty only.

\subsection{Natural Gradient Interpretation and Steepest-Ascent Duality}
\label{app:natgrad}
Let $\langle u,v\rangle_{F}:=u^\top F v$ and its dual norm $\|g\|_{F^{-1}}$.
The maximizer in Lemma~\ref{lem:inner-max-linear} aligns with the natural gradient $v=F^{-1}g$:
\[
\Delta^\star = \arg\max_{\|\Delta\|_F\le \sqrt{2\rho}} g^\top \Delta
= \sqrt{2\rho}\, \frac{v}{\sqrt{g^\top v}}.
\]
Hence, KL--SAM’s inner ascent direction is the \emph{steepest} ascent in the KL geometry; the outer descent step then minimizes the robustified objective.

\subsection{Remainder Bounds and Scaling with \texorpdfstring{$\rho$}{rho}}
\label{app:remainder}
From Section~\ref{app:proof-thm1}, $R_3(\Delta^\star)=\mathcal{O}(\rho^{3/2})$; more explicitly, using the Lipschitz Hessian constant $L_3$,
\[
|R_3(\Delta^\star)| \;\le\; \frac{L_3}{6}\,\|\Delta^\star\|^3
\;\le\; \frac{L_3}{6}\,\left(\sqrt{2\rho}\,\frac{\|F^{-1}g\|}{\|g\|_{F^{-1}}}\right)^3
\;=\; \mathcal{O}(\rho^{3/2}).
\]
Thus the ordering of terms near $\rho=0$ is:
mean term $\mathcal{O}(1)$, risk (std) term $\mathcal{O}(\sqrt{\rho})$, curvature $\mathcal{O}(\rho)$, remainder $o(\rho)$.

\subsection{Cost-SAM vs.\ Lagrangian-SAM: Gradients and Mixed Geometry}
\label{app:which-loss-details}
For Lagrangian-SAM, $g_\lambda=\nabla_\theta \mathcal{L}_\lambda = -\nabla J_r + \lambda \nabla J_c$, so the penalty uses
$\|g_\lambda\|_{F^{-1}}$ and is thus sensitive to the dual variable $\lambda$.
For Cost-SAM, the penalty reduces to $\|\nabla J_c\|_{F^{-1}}$, directly prioritizing directions where cost gradients are large under epistemic uncertainty.
Both share the same Fisher geometry $F$ imposed by the policy class and data; in practice one may compute $F$ from the actor and re-use it for either choice.

\subsection{Practical Computation: Fisher--Vector Products and Conjugate Gradient}
\label{app:fvp}
Given a batch of state--action pairs $(s_i,a_i)$, the empirical Fisher--vector product is
\[
(Fv) \;\approx\; \frac{1}{N}\sum_{i=1}^N \big(\nabla_\theta \log \pi_\theta(a_i\mid s_i)^\top v\big)\, \nabla_\theta \log \pi_\theta(a_i\mid s_i) \;+\; \varepsilon v,
\]
with damping $\varepsilon$. Conjugate gradient (CG) solves $F v \approx g$ up to a tolerance.
The inner point is then
\[
\Delta^\star = \sqrt{2\rho}\,\frac{v}{\sqrt{g^\top v}},
\]
which enforces $\tfrac{1}{2}\Delta^{\star\top}F\Delta^\star=\rho$ exactly even if $v$ is an \emph{inexact} natural gradient (since the normalization uses the current $g^\top v$).

\subsection{Full Second-Order Inner Solver (Optional)}
\label{app:optional-secondorder}
If one wishes to incorporate curvature into the inner ascent (useful when $\rho$ is not very small), solve the trust-region system
\[
(H - \eta F)\,\Delta \;=\; -g, \qquad \text{with }\eta>\lambda_{\max}(M).
\]
A safeguarded Newton or bisection on $\eta$ can enforce the boundary condition $\tfrac{1}{2}\Delta^\top F \Delta=\rho$.
This requires the same primitives as TRPO (Fisher–vector and Hessian–vector products via automatic differentiation).

\subsection{Link to Amount of Risk-Aversion}
\label{app:amount}
Combining Sections~\ref{app:prelim}--\ref{app:credible}, the robust objective near $\theta$ is
\[
\mathcal{R}_\rho(\theta) \;=\; \mathcal{L}_\lambda(\theta) \;+\; \underbrace{\sqrt{2\rho}}_{\beta(\rho)}\;\underbrace{\|g(\theta)\|_{F(\theta)^{-1}}}_{\sigma_{\mathrm{epi}}(\theta)} \;+\; \mathcal{O}(\rho),
\]
and under a Gaussian credible level $\alpha_{\mathrm{cov}}$ (coverage), $\rho=\tfrac{1}{2}\chi^2_p(\alpha_{\mathrm{cov}})$ yields $\beta(\rho)=\sqrt{\chi^2_p(\alpha_{\mathrm{cov}})}$.
Thus $\rho$ implements a tunable epistemic risk aversion coefficient $\beta(\rho)$ with a clear Bayesian calibration.

\subsection{Finite-Sample and Damping Effects (Informal)}
\label{app:finite-sample}
With finite data, $F$ fluctuates and damping $\varepsilon I$ is standard. Replacing $F$ by $F_\varepsilon$ preserves all derivations with $\|g\|_{F^{-1}}$ replaced by $\|g\|_{F_\varepsilon^{-1}}$. Credible-set calibration then uses $\chi^2_{p}$ with an ``effective'' dimension if strong regularization reduces rank; in practice we keep the mapping as a heuristic that is exact in the large-sample Laplace limit.

\subsection{Summary}
\label{app:summary}
KL--SAM’s inner maximization is the support function of a Fisher ellipsoid, producing a \emph{mean + $\beta$·(epistemic std)} robust loss with $\beta(\rho)=\sqrt{2\rho}$, curvature corrections bounded by $\rho\|F^{-1/2}HF^{-1/2}\|$, and a Bayesian calibration $\rho=\tfrac12 \chi^2_p(\alpha_{\mathrm{cov}})$. These identities justify both the interpretation and the implementation of KL--SAM in policy optimization under safety constraints.



\section{Block-Coordinate KL--SAM: Equivalence to Joint Penalty to First Order}
\label{app:block-sam}

\subsection{Setup}
Let $w=(\theta,\phi)$ and $\mathcal{L}_\lambda(w)$ be $C^2$ with locally Lipschitz Hessian. Define block metrics
\[
\Sigma(w)^{-1} \;=\; \mathrm{diag}\!\big(F_\theta(\theta),\,G_\phi(\phi)\big),
\]
with $F_\theta\succ 0$ the policy Fisher and $G_\phi\succ 0$ a Gauss--Newton/Fisher for the critic. One \emph{block-coordinate} KL--SAM cycle consists of:
\begin{align*}
\text{(Actor step)}\quad 
&\Delta_\theta^\star \;=\; \arg\max_{\tfrac{1}{2}\Delta_\theta^\top F_\theta \Delta_\theta \le \rho_\theta}\;\mathcal{L}_\lambda(\theta+\Delta_\theta,\phi), 
\qquad (\theta \leftarrow \theta+\Delta_\theta^\star),\\
\text{(Critic step)}\quad 
&\Delta_\phi^\star \;=\; \arg\max_{\tfrac{1}{2}\Delta_\phi^\top G_\phi \Delta_\phi \le \rho_\phi}\;\mathcal{L}_\lambda(\theta,\phi+\Delta_\phi),
\qquad (\phi \leftarrow \phi+\Delta_\phi^\star).
\end{align*}

\subsection{Main proposition}
\begin{proposition}[Alternating equals joint to first order]
\label{prop:block-eq}
Let $g_\theta=\nabla_\theta \mathcal{L}_\lambda(\theta,\phi)$, $g_\phi=\nabla_\phi \mathcal{L}_\lambda(\theta,\phi)$, and partition the Hessian
$H=\nabla^2_w \mathcal{L}_\lambda = \begin{psmallmatrix} H_{\theta\theta} & H_{\theta\phi}\\ H_{\phi\theta} & H_{\phi\phi}\end{psmallmatrix}$.
Assume the local KL expansions and Lipschitz-Hessian conditions in App.~\ref{app:assumptions}.
Then the increase in the objective across one full block cycle satisfies
\begin{equation}
\label{eq:block-first-order}
\mathcal{L}_\lambda(\theta+\Delta_\theta^\star,\phi+\Delta_\phi^\star)
= \mathcal{L}_\lambda(\theta,\phi)
+ \sqrt{2\rho_\theta}\,\|g_\theta\|_{F_\theta^{-1}}
+ \sqrt{2\rho_\phi}\,\|g_\phi\|_{G_\phi^{-1}}
+ R_{\mathrm{curv}} + R_{\mathrm{cpl}},
\end{equation}
with curvature remainder $|R_{\mathrm{curv}}|\le C_1\,(\rho_\theta+\rho_\phi)$ and coupling remainder
\begin{equation}
\label{eq:block-coupling}
|R_{\mathrm{cpl}}|
\;\le\;
2\,\sqrt{\rho_\theta \rho_\phi}\;\big\|\,G_\phi^{-1/2}\,H_{\phi\theta}\,F_\theta^{-1/2}\big\| \;+\; \mathcal{O}\!\big(\rho_\theta^{3/2}+\rho_\phi^{3/2}\big).
\end{equation}
Consequently, as $\rho_\theta,\rho_\phi\to 0$, the alternating scheme matches the joint mean--std penalty to first order $\mathcal{O}(\sqrt{\rho_\theta})+\mathcal{O}(\sqrt{\rho_\phi})$.
\end{proposition}

\paragraph{Remarks.}
(i) If actor and critic share no parameters (so $H_{\phi\theta}=0$), the coupling term vanishes and the first-order penalties \emph{add exactly} up to curvature $\mathcal{O}(\rho)$.
(ii) Setting $\rho_\theta=\rho_\phi=\rho$ makes $R_{\mathrm{cpl}}=\mathcal{O}(\rho)$, strictly lower order than the $\mathcal{O}(\sqrt{\rho})$ penalties.

\subsection{Proof of Proposition~\ref{prop:block-eq}}
\begin{proof}
\textbf{Actor step.} Linearize in $\Delta_\theta$ keeping $\phi$ fixed:
\[
\mathcal{L}_\lambda(\theta+\Delta_\theta,\phi) 
= \mathcal{L}_\lambda(\theta,\phi) + g_\theta^\top \Delta_\theta + \tfrac{1}{2}\Delta_\theta^\top H_{\theta\theta}\Delta_\theta + R_\theta(\Delta_\theta).
\]
By Lemma~\ref{lem:inner-max-linear}, the maximizer under $\tfrac{1}{2}\Delta_\theta^\top F_\theta \Delta_\theta\le \rho_\theta$ is
$\Delta_\theta^\star = \sqrt{2\rho_\theta}\,F_\theta^{-1}g_\theta / \|g_\theta\|_{F_\theta^{-1}}$ with value
$\sqrt{2\rho_\theta}\,\|g_\theta\|_{F_\theta^{-1}} + \tfrac{1}{2}\Delta_\theta^{\star\top} H_{\theta\theta}\Delta_\theta^\star + R_\theta(\Delta_\theta^\star)$.
Using Lipschitz-Hessian, $R_\theta(\Delta_\theta^\star)=\mathcal{O}(\rho_\theta^{3/2})$, and
$\tfrac{1}{2}\Delta_\theta^{\star\top} H_{\theta\theta}\Delta_\theta^\star=\mathcal{O}(\rho_\theta)$.

\textbf{Critic step.} Now expand around $(\theta+\Delta_\theta^\star,\phi)$:
\[
\mathcal{L}_\lambda(\theta+\Delta_\theta^\star,\phi+\Delta_\phi)
= \mathcal{L}_\lambda(\theta+\Delta_\theta^\star,\phi)
+ \underbrace{\big(g_\phi + H_{\phi\theta}\Delta_\theta^\star\big)^\top \Delta_\phi}_{\text{linear term in }\Delta_\phi}
+ \tfrac{1}{2}\Delta_\phi^\top H_{\phi\phi}\Delta_\phi
+ R_\phi(\Delta_\phi;\Delta_\theta^\star).
\]
Maximizing the linear term over $\{\tfrac{1}{2}\Delta_\phi^\top G_\phi \Delta_\phi \le \rho_\phi\}$ yields (again by Lemma~\ref{lem:inner-max-linear})
\[
\sqrt{2\rho_\phi}\,\big\|\,g_\phi + H_{\phi\theta}\Delta_\theta^\star\,\big\|_{G_\phi^{-1}}.
\]
Use the triangle inequality in the $G_\phi^{-1}$-norm:
\[
\big\|\,g_\phi + H_{\phi\theta}\Delta_\theta^\star\,\big\|_{G_\phi^{-1}}
\le \|g_\phi\|_{G_\phi^{-1}} + \|H_{\phi\theta}\Delta_\theta^\star\|_{G_\phi^{-1}}
\le \|g_\phi\|_{G_\phi^{-1}} + \big\|G_\phi^{-1/2}H_{\phi\theta}F_\theta^{-1/2}\big\|\,\|F_\theta^{1/2}\Delta_\theta^\star\|.
\]
The actor constraint gives $\|F_\theta^{1/2}\Delta_\theta^\star\|=\sqrt{2\rho_\theta}$, hence
\[
\sqrt{2\rho_\phi}\,\big\|\,g_\phi + H_{\phi\theta}\Delta_\theta^\star\,\big\|_{G_\phi^{-1}}
\le \sqrt{2\rho_\phi}\,\|g_\phi\|_{G_\phi^{-1}} 
+ 2\,\sqrt{\rho_\theta\rho_\phi}\,\big\|G_\phi^{-1/2}H_{\phi\theta}F_\theta^{-1/2}\big\|.
\]
The quadratic and remainder terms in $\Delta_\phi$ contribute $\mathcal{O}(\rho_\phi)$ and $\mathcal{O}(\rho_\phi^{3/2})$, respectively.
Summing the actor and critic contributions yields \eqref{eq:block-first-order} with bounds \eqref{eq:block-coupling}.
\end{proof}



% Requires: amsmath, amssymb
\section*{Actor Update With Critic--SAM: A Compact Derivation}

\paragraph{Setup.}
Let the policy be Gaussian with unit variance,
\(\pi_\theta(a\mid s)=\frac{1}{\sqrt{2\pi}}\exp\!\big(-\tfrac{(a-\mu_\theta(s))^2}{2}\big)\).
A single-sample actor update at \(\theta=\theta^0\) driven by an advantage estimate
\(A_\phi(s,a)\) is
\begin{equation}
U(s,a)\;=\;A_\phi(s,a)\,\nabla_{\theta}\log\pi_{\theta}(a\mid s)\Big|_{\theta=\theta^0}
\;=\;A_\phi(s,a)\,(a-\mu_{\theta^0}(s))\,\nabla_{\theta}\mu_\theta(s)\Big|_{\theta=\theta^0}.
\end{equation}
Under the simplifying assumption \(\mu_\theta(s)=\theta_s\) (one parameter per state),
\(\nabla_\theta\mu_\theta(s)=1\) and
\begin{equation}
U(s,a)\;=\;A_\phi(s,a)\,(a-\theta^0_s).
\end{equation}

\subsection*{Critic SAM}
Consider a value critic \(V_\phi\) trained by the squared TD loss
\begin{equation}
\mathcal{L}_c(\phi)\;=\;\tfrac12\,\delta_\phi^2,\qquad
\delta_\phi\;\qquad\;r(s,a)+\gamma V_\phi(s')-V_\phi(s).
\end{equation}
A (first-order) SAM perturbation for a minimization problem chooses
\begin{equation}
\tilde{\phi}\;=\;\phi\;+\;\rho\,
\frac{\nabla_\phi \mathcal{L}_c(\phi)}{\big\|\nabla_\phi \mathcal{L}_c(\phi)\big\|}
\;=\;\phi\;+\;\rho\,
\frac{\delta_\phi\,\nabla_\phi \delta_\phi}{\big\|\delta_\phi\,\nabla_\phi \delta_\phi\big\|}
\;=\;\phi\;+\;\rho\,\operatorname{sign}(\delta_\phi)\,
\frac{\nabla_\phi \delta_\phi}{\|\nabla_\phi \delta_\phi\|},
\end{equation}
and updates the critic using the gradient at \(\tilde{\phi}\).
A first-order Taylor expansion of \(\delta\) along this direction yields
\begin{equation}
\delta_{\tilde{\phi}}
\;\approx\;
\delta_\phi\;+\;\nabla_\phi \delta_\phi^\top\!\left(
\rho\,\operatorname{sign}(\delta_\phi)\,\frac{\nabla_\phi \delta_\phi}{\|\nabla_\phi \delta_\phi\|}
\right)
\;=\;\delta_\phi\;+\;\rho\,\operatorname{sign}(\delta_\phi)\,\|\nabla_\phi \delta_\phi\|.
\label{eq:delta-tilde}
\end{equation}
Hence, whenever \(\delta_\phi\neq 0\),
\(|\delta_{\tilde{\phi}}|\approx |\delta_\phi|+\rho\,\|\nabla_\phi \delta_\phi\|\) strictly increases.

\paragraph{Impact on the actor update.}
If the actor uses the SAM-perturbed critic to form its advantage,
\(A_{\tilde{\phi}}(s,a)=\delta_{\tilde{\phi}}(s,a,s')\), the per-sample update at \(\theta^0\) becomes
\begin{equation}
U_{\text{SAM-critic}}(s,a)
\;=\;A_{\tilde{\phi}}(s,a)\,(a-\theta^0_s)
\;=\;\delta_{\tilde{\phi}}(s,a,s')\,(a-\theta^0_s).
\end{equation}
Thus the (per-sample) scaling induced by critic SAM is
\begin{equation}
\frac{U_{\text{SAM-critic}}(s,a)}{U(s,a)}
\;=\;\frac{\delta_{\tilde{\phi}}}{\delta_\phi}
\;\approx\;1+\rho\,\frac{\|\nabla_\phi \delta_\phi\|}{|\delta_\phi|}\;>\;1
\qquad(\delta_\phi\neq 0).
\label{eq:scaling}
\end{equation}
In words: critic SAM \emph{uniformly magnifies} the magnitude of the actor update,
with amplification proportional to a sharpness proxy \(\|\nabla_\phi \delta_\phi\|\).

\subsection*{Concrete illustration: one parameter per state}
Let \(V_\phi(s)=\phi_s\). Then
\begin{equation}
\delta_\phi=r+\gamma\phi_{s'}-\phi_s,\qquad
\nabla_\phi\delta_\phi=\gamma\,e_{s'}-e_s,
\qquad \big\|\nabla_\phi\delta_\phi\big\|=\sqrt{1+\gamma^2}.
\end{equation}
Plugging into \eqref{eq:delta-tilde} and \eqref{eq:scaling} gives
\begin{equation}
\delta_{\tilde{\phi}}
\;\approx\;\delta_\phi+\rho\,\operatorname{sign}(\delta_\phi)\sqrt{1+\gamma^2},
\qquad
\boxed{\;
\frac{U_{\text{SAM-critic}}(s,a)}{U(s,a)}
\;\approx\;1+\rho\,\frac{\sqrt{1+\gamma^2}}{|\delta_\phi|}
\;}
\end{equation}
which is larger when \(|\delta_\phi|\) is small (more uncertainty) or when \(\gamma\) is large
(stronger bootstrapping).

\subsection*{CMDP / Lagrangian actor with reward and cost critics}
For constrained RL with a Lagrangian actor update,
\begin{equation}
U(s,a)
\;=\;\big(A^R_\phi(s,a)-\lambda\,A^C_\psi(s,a)\big)\,(a-\theta^0_s),
\end{equation}
applying SAM \emph{only} to the cost critic yields
\begin{align}
U_{\text{SAM-}C}(s,a)
&=\Big(A^R_\phi(s,a)-\lambda\,A^C_{\tilde{\psi}}(s,a)\Big)\,(a-\theta^0_s),
\\
A^C_{\tilde{\psi}}(s,a)
&\approx A^C_\psi(s,a)\;+\;\rho_C\,
\operatorname{sign}\big(A^C_\psi(s,a)\big)\,\big\|\nabla_\psi \delta^C_\psi\big\|.
\end{align}
Consequently,
\begin{itemize}
\item If \(A^C_\psi(s,a)>0\) (locally unsafe), the penalty \(-\lambda A^C\) becomes more negative,
further \emph{decreasing} the action likelihood.
\item If \(A^C_\psi(s,a)<0\) (locally safe), the penalty becomes less negative (or positive),
further \emph{increasing} the action likelihood.
\end{itemize}
Thus, cost-critic SAM strengthens safety shaping \emph{most} where the cost critic is sharp/uncertain.

\subsection*{Combining actor and critic SAM}
If SAM is also applied on the actor (with perturbed \(\tilde{\theta}\) and the standard
Gaussian/unit-variance setting),
\begin{equation}
U_{\text{both}}(s,a)\;=\;
\Big(A^R_{\tilde{\phi}}(s,a)-\lambda A^C_{\tilde{\psi}}(s,a)\Big)\,
\frac{\pi_{\tilde{\theta}}(a\mid s)}{\pi_{\theta^0}(a\mid s)}\,
\big(a-\tilde{\theta}_s\big),
\end{equation}
recovering the known actor-side reweighting
(\(\pi_{\tilde{\theta}}/\pi_{\theta^0}\) and \(a-\tilde{\theta}_s\)) together with the
critic-side amplification of advantage magnitudes.

\subsection*{GAE remark}
With generalized advantage estimation,
\begin{equation}
A_\phi^{\text{GAE}}(s_t,a_t)
=\sum_{k\ge 0}(\gamma\lambda)^k\,\delta_\phi^{(t+k)},
\qquad
\delta_\phi^{(t)}=r_t+\gamma V_\phi(s_{t+1})-V_\phi(s_t),
\end{equation}
and the same first-order SAM approximation per step,
\(\delta_{\tilde{\phi}}^{(t)}\approx \delta_\phi^{(t)}+
\rho\,\operatorname{sign}(\delta_\phi^{(t)})\|\nabla_\phi \delta_\phi^{(t)}\|\),
we obtain
\begin{equation}
\big|A_{\tilde{\phi}}^{\text{GAE}}\big|
\;\gtrsim\;
\big|A_\phi^{\text{GAE}}\big|
+\rho\sum_{k\ge 0}(\gamma\lambda)^k\,
\big\|\nabla_\phi \delta_\phi^{(t+k)}\big\|,
\end{equation}
so the amplification-by-sharpness conclusion carries over to GAE.

\subsection*{Summary}
\begin{itemize}
\item \textbf{Actor SAM} (unit-variance Gaussian) asymmetrically reweights gradients:
shrinking positive-advantage pushes and inflating negative-advantage pulls.
\item \textbf{Critic SAM} \emph{uniformly magnifies} advantage magnitudes, with strength
proportional to \(\|\nabla_\phi \delta_\phi\|\), a proxy for epistemic uncertainty.
\item \textbf{Safe RL}: applying SAM on the \emph{cost critic} magnifies avoidance of unsafe
actions and promotion of safer ones, especially where the cost critic is uncertain.
\end{itemize}




\paragraph{Setup.}
Let $\ell(\theta)$ denote a scalar loss we wish to \emph{minimize}. (For maximization of a reward surrogate $f(\theta)$, set $\ell(\theta)=-f(\theta)$.) 
Let $F(\theta)$ be the Fisher information (TRPO geometry), and let the SAM--KL adversary choose a perturbation 
$\Delta \in \mathbb{R}^d$ in the local ellipsoid 
$\mathcal{E}_\rho := \{\Delta : \Delta^\top F(\theta)\,\Delta \le \rho^2\}$.
The one-step SAM objective is
\[
\mathsf{SAM}_\rho(\theta) \;:=\; \sup_{\Delta \in \mathcal{E}_\rho} \,\ell(\theta+\Delta).
\]
We interpret \emph{epistemic uncertainty} locally as a random parameter perturbation 
$\Delta \sim \mathsf{Law}(\Delta)$ with $\mathbb{E}[\Delta]=0$ and covariance $\mathrm{Cov}(\Delta)=\Sigma$. 
In TRPO geometry we take $\Sigma=F(\theta)^{-1}$. 

\paragraph{Linearization and local smoothness.}
Assume $\ell$ is twice differentiable and \emph{relatively smooth} w.r.t.\ $F(\theta)$:
there exists $L_H \ge 0$ such that for all $\Delta$ in a neighborhood,
$\bigl|\Delta^\top \nabla^2 \ell(\theta+\tau\Delta)\,\Delta\bigr|\le L_H\,\Delta^\top F(\theta)\,\Delta$ for all $\tau\in[0,1]$.
Then the second-order Taylor remainder is controlled as
\[
\ell(\theta+\Delta)=\ell(\theta)+\nabla\ell(\theta)^\top \Delta \;+\; R(\Delta),
\qquad |R(\Delta)|\le \tfrac{L_H}{2}\,\Delta^\top F(\theta)\,\Delta.
\]

\begin{lemma}[SAM is the support function of the epistemic ellipsoid]
\label{lem:support}
Under the above assumptions,
\[
\sup_{\Delta\in\mathcal{E}_\rho}\bigl(\ell(\theta)+\nabla\ell(\theta)^\top \Delta\bigr)
\;=\; \ell(\theta) + \rho \,\|\nabla\ell(\theta)\|_{F(\theta)^{-1}},
\]
where $\|v\|_{F^{-1}}:=\sqrt{v^\top F^{-1} v}$. 
Moreover,
\[
\ell(\theta) + \rho \,\|\nabla\ell\|_{F^{-1}} \;-\; \tfrac{L_H}{2}\rho^2 
\;\le\; \mathsf{SAM}_\rho(\theta) \;\le\; 
\ell(\theta) + \rho \,\|\nabla\ell\|_{F^{-1}} \;+\; \tfrac{L_H}{2}\rho^2 .
\]
\emph{Proof.}
The linear part is the support function of $\mathcal{E}_\rho$; by Cauchy--Schwarz in the Mahalanobis norm,
$\sup_{\Delta^\top F \Delta \le \rho^2} \nabla\ell^\top \Delta = \rho \|\nabla\ell\|_{F^{-1}}$,
attained at $\Delta^\star = \rho\,\frac{F^{-1}\nabla\ell}{\|\nabla\ell\|_{F^{-1}}}$.
The remainder bounds follow from the relative smoothness bound on $R(\Delta)$. \qed
\end{lemma}

\paragraph{Epistemic linear model.}
Model parameter epistemics locally as $\Delta \sim \mathcal{N}(0,\Sigma)$ with $\Sigma=F^{-1}$. 
Then the \emph{linearized epistemic loss}
\[
\widetilde{L}_{\mathrm{lin}} \;:=\; \ell(\theta) + \nabla\ell(\theta)^\top \Delta
\]
is Gaussian with mean $\mu=\ell(\theta)$ and variance 
$\sigma^2=\nabla\ell(\theta)^\top \Sigma \,\nabla\ell(\theta)=\|\nabla\ell(\theta)\|_{F^{-1}}^2$.
Let $z_\alpha := \Phi^{-1}(\alpha)$ where $\Phi$ is the standard normal cdf.

\begin{proposition}[SAM equals a VaR distortion of the linearized epistemic loss]
\label{prop:var}
For any $\rho>0$, set $\alpha:=\Phi(\rho)$.
Then
\[
\ell(\theta) + \rho\,\|\nabla\ell(\theta)\|_{F^{-1}}
\;=\; \mathrm{VaR}_\alpha\!\big(\widetilde{L}_{\mathrm{lin}}\big),
\]
i.e., the linearized SAM objective equals the $\alpha$-quantile (a \emph{distortion risk measure}) of the epistemic loss.
Moreover,
\[
\mathrm{VaR}_\alpha\!\big(\widetilde{L}_{\mathrm{lin}}\big)
\;\le\; \mathrm{CVaR}_\alpha\!\big(\widetilde{L}_{\mathrm{lin}}\big)
\;=\; \ell(\theta) + \|\nabla\ell\|_{F^{-1}}\,\frac{\varphi(z_\alpha)}{1-\alpha},
\]
so the SAM value is (for fixed $\alpha$) a lower bound on the coherent distortion $\mathrm{CVaR}_\alpha$.
\emph{Proof.}
For a Gaussian $X\sim\mathcal{N}(\mu,\sigma^2)$, $\mathrm{VaR}_\alpha(X)=\mu+\sigma z_\alpha$; here $\sigma=\|\nabla\ell\|_{F^{-1}}$ and $z_\alpha=\rho$ by construction. The CVaR formula is standard for Gaussians. \qed
\end{proposition}

\begin{theorem}[Pessimism w.r.t.\ epistemic uncertainty]
\label{thm:pessimism}
Under Lemma~\ref{lem:support} and Proposition~\ref{prop:var}, for small enough $\rho$ the SAM objective satisfies
\[
\mathsf{SAM}_\rho(\theta) \;\approx\; \mathrm{VaR}_{\Phi(\rho)}\!\big(\widetilde{L}_{\mathrm{lin}}\big),
\]
up to a second-order error $\pm \tfrac{L_H}{2}\rho^2$. Hence SAM implements a \emph{distortion risk metric} that upweights the worst-case (upper-tail) outcomes of the epistemic loss distribution; larger $\rho$ corresponds to more pessimism (larger quantile). 
Equivalently, for reward maximization with $f=-\ell$,
\[
\underbrace{f(\theta) - \rho\,\|\nabla f(\theta)\|_{F^{-1}}}_{\text{SAM for maximization}}
\;=\; \mathrm{VaR}_{1-\Phi(\rho)}\!\big(\widetilde{F}_{\mathrm{lin}}\big),
\]
the \emph{lower} quantile of the epistemic reward $\widetilde{F}_{\mathrm{lin}} := f(\theta)+\nabla f^\top \Delta$, i.e., pessimism about reward. \qed
\end{theorem}

\paragraph{Specialization to TRPO/PPO surrogates.}
Let $f_{\text{TRPO}}(\theta)=\mathbb{E}\big[r_\theta(s,a)\,\widehat{A}(s,a)\big]$ denote the standard surrogate, e.g.,
$f(\theta)=\mathbb{E}[\,r(\theta)\,\widehat{A}\,]$ with importance ratio $r(\theta)=\pi_\theta(a|s)/\pi_{\theta_0}(a|s)$.
SAM for maximization uses the \emph{worst-case} decrease in $f$ over the KL-ball,
\[
\max_{\theta} \min_{\Delta\,:\,\Delta^\top F\,\Delta\le \rho^2} f(\theta+\Delta)
\;\approx\; \max_\theta \Big\{ f(\theta) - \rho\,\|\nabla f(\theta)\|_{F^{-1}} \Big\}.
\]
By Theorem~\ref{thm:pessimism}, this equals maximizing a chosen lower quantile (VaR) of the linearized epistemic reward, hence is a distortion measure that is \emph{pessimistic} w.r.t.\ epistemic uncertainty.

\paragraph{CMDP Lagrangian.}
For a CMDP with Lagrangian objective $f_\lambda(\theta)=J_r(\theta)-\lambda(J_c(\theta)-\bar{c})$, SAM yields
\[
\max_\theta \min_{\Delta^\top F \Delta \le \rho^2} f_\lambda(\theta+\Delta)
\;\approx\; \max_\theta \Big\{ f_\lambda(\theta) - \rho\,\|\nabla f_\lambda(\theta)\|_{F^{-1}} \Big\}.
\]
If one constructs the adversarial perturbation using the \emph{cost} component only (a common safe-exploration variant), the penalty term grows with $\|\nabla J_c(\theta)\|_{F^{-1}}$, explicitly biasing against policies with high epistemic sensitivity of cost, i.e., \emph{pessimistic w.r.t.\ cost uncertainty}. 

\paragraph{Choosing the ``distortion level''.}
With Fisher geometry $\Sigma=F^{-1}$ and Gaussian local epistemics, the SAM radius maps to a quantile via
\[
\alpha \;=\; \Phi(\rho) 
\qquad(\text{loss}), 
\qquad\text{or}\qquad
\alpha \;=\; 1-\Phi(\rho) 
\qquad(\text{reward}).
\]
In TRPO one often writes the KL trust-region as $\Delta^\top F \Delta \le \varepsilon$; identifying $\rho=\sqrt{\varepsilon}$ selects the distortion level $\alpha=\Phi(\sqrt{\varepsilon})$.

\paragraph{Takeaway.}
Under mild local conditions, SAM with KL/Fisher geometry is \emph{exactly} the VaR distortion of the linearized epistemic objective and, up to a quadratic remainder, a lower/upper bound on CVaR. Thus, SAM provably implements a pessimistic distortion metric w.r.t.\ epistemic uncertainty in our actor (and analogously critic) objectives, explaining its safety-leaning behavior during exploration.


\paragraph{Wang distortion recap.}
For a loss $X$ with cdf $F_X$, the Wang distortion with parameter $\lambda\in\mathbb{R}$ is
\[
g_\lambda(u)\;=\;\Phi\!\big(\Phi^{-1}(u)+\lambda\big),\qquad u\in[0,1],
\]
and the associated distortion risk measure (premium) is 
\[
\rho_W^\lambda(X)\;=\;\int_0^1 F_X^{-1}(u)\, d g_\lambda(u).
\]
Since $g_\lambda$ is increasing and concave, $\rho_W^\lambda$ is a coherent, law-invariant risk measure on $L^\infty$.

\paragraph{Setup.}
Let $\ell(\theta)$ be a twice-differentiable loss and $F(\theta)$ the Fisher metric.
Define the SAM objective over the KL/Fisher ellipsoid $\mathcal{E}_\rho:=\{\Delta:\Delta^\top F(\theta)\Delta\le \rho^2\}$:
\[
\mathsf{SAM}_\rho(\theta)\;=\;\sup_{\Delta\in\mathcal{E}_\rho}\,\ell(\theta+\Delta).
\]
Assume \emph{relative smoothness} w.r.t.\ $F(\theta)$ (as in the main text): for some $L_H\ge0$,
$\bigl|\Delta^\top \nabla^2\ell(\theta+\tau\Delta)\Delta\bigr|\le L_H\,\Delta^\top F(\theta)\Delta$ for $\tau\in[0,1]$.
Let the local epistemic perturbation be $\Delta\sim\mathcal{N}(0,\Sigma)$ with $\Sigma=F(\theta)^{-1}$.
Then the \emph{linearized epistemic loss} is
\[
\widetilde{L}_{\mathrm{lin}}\;:=\;\ell(\theta)+\nabla\ell(\theta)^\top \Delta
\;\sim\;\mathcal{N}\!\bigl(\mu,\sigma^2\bigr),\quad
\mu:=\ell(\theta),\quad \sigma:=\|\nabla\ell(\theta)\|_{F(\theta)^{-1}}.
\]

\begin{lemma}[Closed form of Wang distortion for Gaussian linearization]
\label{lem:wang-gauss}
If $X\sim\mathcal{N}(\mu,\sigma^2)$, then
\[
\rho_W^\lambda(X)\;=\;\mu+\sigma\,\lambda.
\]
\emph{Proof.}
Write $X=\mu+\sigma Z$ with $Z\sim\mathcal{N}(0,1)$. The Wang transform changes tail probabilities via
$\bar F_{X}^{\,W}(x)=g_\lambda(\bar F_X(x))$, which for Gaussian is equivalent to an exponential tilt of $Z$:
$d\mathbb{Q}_\lambda/d\mathbb{P}=\exp(\lambda Z-\tfrac{1}{2}\lambda^2)$, under which $Z\sim\mathcal{N}(\lambda,1)$.
Distortion premium equals expectation under $\mathbb{Q}_\lambda$, so
$\rho_W^\lambda(X)=\mathbb{E}_{\mathbb{Q}_\lambda}[X]=\mu+\sigma\,\mathbb{E}_{\mathbb{Q}_\lambda}[Z]=\mu+\sigma\lambda$. \qed
\end{lemma}

\begin{lemma}[SAM support value with curvature control]
\label{lem:sam-support}
Under relative smoothness,
\[
\ell(\theta)+\sigma\,\rho\;-\;\tfrac{L_H}{2}\rho^2\;\le\;\mathsf{SAM}_\rho(\theta)\;\le\;\ell(\theta)+\sigma\,\rho\;+\;\tfrac{L_H}{2}\rho^2,
\]
with $\sigma=\|\nabla\ell(\theta)\|_{F^{-1}}$. The center term is attained by the linear model and the maximizer
$\Delta^\star=\rho\,\frac{F^{-1}\nabla\ell}{\|\nabla\ell\|_{F^{-1}}}$.
\end{lemma}

\begin{theorem}[SAM $\approx$ Wang distortion (local Gaussian epistemics)]
\label{thm:sam-wang}
With $\widetilde{L}_{\mathrm{lin}}\sim\mathcal{N}(\mu,\sigma^2)$ as above and $\lambda=\rho$,
\[
\mathsf{SAM}_\rho(\theta)\;=\;\rho_W^{\lambda}\!\big(\widetilde{L}_{\mathrm{lin}}\big)\;\pm\;\tfrac{L_H}{2}\rho^2,
\qquad\text{i.e.,}\quad
\mathsf{SAM}_\rho(\theta)\;=\;\mu+\sigma\rho\;\pm\;O(\rho^2).
\]
Thus SAM implements, up to a second-order curvature error, a Wang-type \emph{pessimistic distortion} of the epistemic loss with aversion level $\lambda=\rho$.
\end{theorem}

\paragraph{Reward maximization and CMDP specialization.}
For reward $f=-\ell$ (maximize), Lemma~\ref{lem:wang-gauss} gives
\[
\max_\theta \min_{\Delta^\top F\Delta\le \rho^2} f(\theta+\Delta)
\;\approx\;\max_\theta \Big\{\,\rho_W^{-\rho}\!\big(\widetilde{F}_{\mathrm{lin}}\big)\,\Big\}
\;=\;\max_\theta \Big\{\,f(\theta)-\rho\,\|\nabla f(\theta)\|_{F^{-1}}\,\Big\},
\]
i.e., a Wang distortion with parameter $-\rho$ of the epistemic reward $\widetilde{F}_{\mathrm{lin}}=f(\theta)+\nabla f^\top \Delta$.
For a CMDP Lagrangian $f_\lambda(\theta)=J_r(\theta)-\lambda(J_c(\theta)-\bar c)$, the same reasoning yields
\[
\max_\theta \min_{\Delta^\top F\Delta\le \rho^2} f_\lambda(\theta+\Delta)
\;\approx\;\max_\theta \Big\{\,\rho_W^{-\rho}\!\big(\widetilde{F}_{\lambda,\mathrm{lin}}\big)\,\Big\}
\;=\;\max_\theta \Big\{\,f_\lambda(\theta)-\rho\,\|\nabla f_\lambda(\theta)\|_{F^{-1}}\,\Big\}.
\]
If the inner adversary is cost-only, replace $\|\nabla f_\lambda\|_{F^{-1}}$ by $\|\nabla J_c\|_{F^{-1}}$, yielding explicit pessimism w.r.t.\ \emph{cost} epistemics.

\paragraph{Relation to VaR/CVaR and choice of $\rho$.}
For Gaussian $X$, $\mathrm{VaR}_\alpha(X)=\mu+\sigma z_\alpha$ with $z_\alpha=\Phi^{-1}(\alpha)$ and 
$\mathrm{CVaR}_\alpha(X)=\mu+\sigma\,\frac{\varphi(z_\alpha)}{1-\alpha}$.
Choosing $\alpha=\Phi(\rho)$ makes
\[
\rho_W^\rho(X)=\mu+\sigma\rho=\mathrm{VaR}_{\Phi(\rho)}(X)\;\le\;\mathrm{CVaR}_{\Phi(\rho)}(X),
\]
so the Wang distortion coincides numerically with the matching Gaussian VaR and sits below CVaR. 
In TRPO, a KL budget $\varepsilon$ corresponds to $\rho=\sqrt{\varepsilon}$, hence $\lambda=\sqrt{\varepsilon}$.

\paragraph{Beyond Gaussian.}
If $\Delta$ is \emph{elliptical} with scatter $F^{-1}$, the linearized loss remains location-scale: 
$\widetilde{L}_{\mathrm{lin}}=\mu+\sigma Z$ where $Z$ is symmetric. Then
\[
\rho_W^\lambda(\widetilde{L}_{\mathrm{lin}})=\mu+\sigma\,\kappa_Z(\lambda),\quad 
\kappa_Z(\lambda):=\int_0^1 H_Z^{-1}(u)\, d\Phi\!\big(\Phi^{-1}(u)+\lambda\big),
\]
recovering $\kappa_Z(\lambda)=\lambda$ for Gaussian $Z$. 
Lemma~\ref{lem:sam-support} still gives $\mathsf{SAM}_\rho(\theta)=\mu+\sigma\rho\pm O(\rho^2)$,
so SAM matches the Wang distortion at \emph{first order} and remains a calibrated, pessimistic distortion in general elliptical models.
